# Supplementary material for: ELUQuant: Event-Level Uncertainty Quantification in Deep Inelastic Scattering
Source: arXiv:2310.02913 source file (2023-10-04)
Supplement: Supplementary file 1 [file 6_Appendix.tex]

%\newpage
\appendix

\section{Title Here} \label{app:complete}
